# Supplementary material for: Skyrmion motion in magnetic anisotropy gradients: Acceleration caused by deformation
Source: arXiv:2308.11361 source file (2023-08-22)
Supplement: Supplementary file 1 [file appendix.tex]

\appendix

\section{A1}

Appendix here
